# Supplementary material for: Active Domain Adaptation for mmWave-based HAR via Renyi Entropy-based Uncertainty Estimation
Source: arXiv:2511.04219 source file (2025-11-06)
Supplement: Supplementary file 1 [file appendix.tex]

\appendices

\section{Derivations for R$\acute{e}$nyi Entropy-based Uncertainty Measures}\label{app:proofs}

This appendix details the derivations for quantifying domain uncertainty (\Equation{domain_uncertainty}) and prediction uncertainty (\Equation{predictive_uncertainty}).
In \Section{uncertainty}, we adopt Hayashi's definition of mutual information of order $s$ and R$\acute{e}$nyi conditional entropy to measure these uncertainties.
When $\boldsymbol{\omega}$ is a continuous random variable and $\boldsymbol{\mu}$ is a discrete random variable, the formulation follows \Equation{conditional_entropy} in \cite{hayashi2011exponential, kamatsuka2025several}. 

\begin{small}
\begin{equation}
    \label{eq:conditional_entropy}
    H_s(\boldsymbol{\omega} \mid \boldsymbol{\mu}) = \frac{1}{1-s} \log \left( \int_{\boldsymbol{\mu}} p_{\boldsymbol{\mu}}(\boldsymbol{\mu}) \sum_{c=1}^n p_{\boldsymbol{\omega} \mid \boldsymbol{\mu}}(\boldsymbol{\omega} \mid \boldsymbol{\mu})^s d\boldsymbol{\mu} \right),
\end{equation}
\end{small}
\begin{equation}
    I_s(\boldsymbol{\omega} \mid \boldsymbol{\mu}) = H_s(\boldsymbol{\omega}) - H_s(\boldsymbol{\omega} \mid \boldsymbol{\mu}),
\end{equation}

where $H_s(\boldsymbol{\omega})$ denotes the R$\acute{e}$nyi entropy of $\boldsymbol{\omega}$, while $I_s(\boldsymbol{\omega} \mid \boldsymbol{\mu})$ and $H_s(\boldsymbol{\omega} \mid \boldsymbol{\mu})$ denote the R$\acute{e}$nyi mutual information and conditional entropy between $\boldsymbol{\omega}$ and $\boldsymbol{\mu}$, respectively.
As discussed in \Section{dpn}, $\boldsymbol{\omega}$ follows a Dirichlet distribution (\Equation{Dirichlet}) and $\boldsymbol{\omega} \mid \boldsymbol{\mu}$ follows a categorical distribution (\Equation{mu}). Therefore, \textbf{the conditional entropy (\Equation{conditional_entropy})} can be derived as follows:

\begin{footnotesize}
\begin{equation}
    \label{eq:conditional_entropy_2}
    \begin{split}
        \mathcal{U}_{\text {pred}}(x)&=H_s(\boldsymbol{\omega} \mid \boldsymbol{\mu})\\
         &=\frac{1}{1-s} \log \left( \int_{\boldsymbol{\mu}} \frac{\Gamma(\alpha_0)}{\prod_{i=1}^{n}\Gamma(\alpha_i)} \prod_{i=1}^n \boldsymbol{\mu}_i^{\alpha_i-1} \sum_{c=1}^n \boldsymbol{\mu}_c^s d\boldsymbol{\mu} \right) \\
        &=\frac{1}{1-s} \log \left( \sum_{c=1}^n \frac{\Gamma(\alpha_0)}{\prod_{i=1}^{n}\Gamma(\alpha_i)} \int_{\boldsymbol{\mu}} (\prod_{i=1,i \neq c}^n \boldsymbol{\mu}_i^{\alpha_i-1})\boldsymbol{\mu}_c^{\alpha_c+s-1}  d\boldsymbol{\mu} \right) \\
        &=\frac{1}{1-s} \log \left( \sum_{c=1}^n \frac{\Gamma(\alpha_0)}{\prod_{i=1}^{n}\Gamma(\alpha_i)} \frac{\prod_{i=1,i\neq c}^{n}\Gamma(\alpha_i)}{\Gamma(\alpha_0+s)}\Gamma(\alpha_c+s)   \right) \\
        &=\frac{1}{1-s} \log \left( \sum_{c=1}^n \frac{\Gamma(\alpha_0)\Gamma(\alpha_c+s)}{\Gamma(\alpha_c)\Gamma(\alpha_0+s)} \right).
    \end{split}
\end{equation}
\end{footnotesize}

By combining \Equation{renyi_entropy} and \Equation{posterior}, the R$\acute{e}$nyi entropy of $\boldsymbol{\omega}$ can be calculated as:
\begin{equation}
    \label{eq:renyi_entropy_2}
    \begin{split}
        H_s\left(\boldsymbol{\omega}\right) &= \frac{1}{1-s} \log \left( \sum_{c=1}^{n} P(\boldsymbol{\omega}_c)^s \right)\\
        &= \frac{1}{1-s} \log \left( \sum_{c=1}^{n} (\frac{\alpha_c}{\alpha_0})^s \right).
    \end{split}
\end{equation} 

Similarly, using \Equation{conditional_entropy_2} and \Equation{renyi_entropy_2}, \textbf{the R$\acute{e}$nyi mutual information} can be computed as:

\begin{footnotesize}
\begin{equation}
    \begin{split}
        \mathcal{U}_{\text {dom}}(x) &= I_s(\boldsymbol{\omega} \mid \boldsymbol{\mu}) \\
        &= H_s(\boldsymbol{\omega}) - H_s(\boldsymbol{\omega} \mid \boldsymbol{\mu})\\
        &= \frac{1}{1-s} \log \left( \sum_{c=1}^{n} (\frac{\alpha_c}{\alpha_0})^s \right) - \frac{1}{1-s} \log \left( \sum_{c=1}^n \frac{\Gamma(\alpha_0)\Gamma(\alpha_c+s)}{\Gamma(\alpha_c)\Gamma(\alpha_0+s)} \right).
    \end{split}
\end{equation} 
\end{footnotesize}

\begin{proof}
We prove that $\mathcal{U}_{\text {dom}}(x) >= 0 $. 

As established in~\cite{artin2015gamma}, $\Gamma(x)$ is given by \Equation{gamma}:
\begin{equation}
    \label{eq:gamma}
    \Gamma(x)=\sqrt{2 \pi} x^{x-\frac{1}{2}} e^{-x+\mu(x)},
\end{equation} 
where $\mu(x)=\frac{\theta}{12x}$ with $0<\theta<1$ is a negligible term when $x$ is large. Based on this, we can deduce \Equation{gamma_gamma}:
\begin{equation}
    \label{eq:gamma_gamma}
    \begin{split}
        \frac{\Gamma(x+s)}{\Gamma(x)} &= \frac{\sqrt{2 \pi} (x+s)^{x+s-\frac{1}{2}} e^{-x-s}}{\sqrt{2 \pi} x^{x-\frac{1}{2}} e^{-x}}\\
        &= x^s (1+\frac{s}{x})^{x+s-\frac{1}{2}}e^{-s}.
    \end{split}
\end{equation}
Since $(1+\frac{s}{x})^{x+s-\frac{1}{2}}$ increases with $x$ and $0<\alpha_c<\alpha_0$, we have:
\begin{equation}
    \begin{split}
        \frac{\Gamma(\alpha_0)\Gamma(\alpha_c+s)}{\Gamma(\alpha_c)\Gamma(\alpha_0+s)} &= \frac{\alpha_c^s (1+\frac{s}{\alpha_c})^{\alpha_c+s-\frac{1}{2}}e^{-s}}{\alpha_0^s (1+\frac{s}{\alpha_0})^{\alpha_0+s-\frac{1}{2}}e^{-s}}\\
        &= \frac{\alpha_c^s}{\alpha_0^s} \frac{(1+\frac{s}{\alpha_c})^{\alpha_c+s-\frac{1}{2}}}{(1+\frac{s}{\alpha_0})^{\alpha_0+s-\frac{1}{2}}}\\
        &\le (\frac{\alpha_c}{\alpha_0})^s.
    \end{split}
\end{equation}
The equality holds when $\alpha_c \rightarrow \infty$ and $\alpha_0 \rightarrow \infty$, or when $\alpha_c = \alpha_0$, \ie, the Dirichlet distribution is sharp, which means EAR has high confidence in the sample.

To sum up, 

\begin{footnotesize}
\begin{equation}
    \begin{split}
        \mathcal{U}_{\text {dom}}(x) &= \frac{1}{1-s} \log \left( \sum_{c=1}^{n} (\frac{\alpha_c}{\alpha_0})^s \right) - \frac{1}{1-s} \log \left( \sum_{c=1}^n \frac{\Gamma(\alpha_0)\Gamma(\alpha_c+s)}{\Gamma(\alpha_c)\Gamma(\alpha_0+s)} \right) \\
        & \ge \frac{1}{1-s} \log \left( \sum_{c=1}^{n} (\frac{\alpha_c}{\alpha_0})^s \right) - \frac{1}{1-s} \log \left( \sum_{c=1}^{n} (\frac{\alpha_c}{\alpha_0})^s \right)\\
        &=0.
    \end{split}
\end{equation}
\end{footnotesize} 

\end{proof}

Therefore, domain uncertainty should always be non-negative in \system. However, due to numerical computation errors, particularly in evaluating the gamma function, it may occasionally result in negative values.

\section{The Distance Upper Bound $\overline{d}(i, j)$ in \Equation{similarity_score}}\label{app:upper_bound}

The distance upper bound $\overline{d}(i, j)$ is determined using the 3-sigma principle, which is defined as:
\begin{equation}
    \label{eq:d_upperbound}
    % \begin{aligned}
    \begin{split}
    \overline{d}(i, j)  &= \begin{cases}
         \mu(j;\mathcal{D}_S) - 3*\sigma(j;\mathcal{D}_S), &  x_j \in \mathcal{D}_S \\
        \mu(j;\mathcal{D}_{Tl}) - 3*\sigma(j;\mathcal{D}_{Tl}), &  x_j \in \mathcal{D}_{Tl}    
         \end{cases}\\
        where\\ 
    \mu(j;\mathcal{D}) &= \frac{1}{\left| \mathcal{D} \right|} \sum_{x_p \in \mathcal{D}} d(j, p)\\
    \sigma(j;\mathcal{D}) &= \sqrt{\frac{1}{\left| \mathcal{D} \right|} \sum_{x_p \in \mathcal{D}}\left(d(j, p)-\frac{1}{\left| \mathcal{D} \right|} \sum_{x_p \in \mathcal{D}} d(j, p)\right)^{2}}
     \end{split}
    % \end{aligned}
\end{equation}
